# Supplementary material for: Minimizing the time-dependent density functional error in Ehrenfest dynamics
Source: arXiv:2106.13752 source file (2021-06-29)
Supplement: Supplementary file 1 [file supmat.pdf]

# **Supplementary Material for "Minimizing the time-dependent density functional error in Ehrenfest dynamics"**

Lionel Lacombe<sup>1</sup> and Neepta T. Maitra<sup>1</sup>

<sup>1</sup>*Department of Physics, Rutgers University, Newark 07102, New Jersey USA*  
(Dated: June 15, 2021)

## I. HAMILTONIAN

In atomic units ( $e^2 = \hbar = m_e = 1$ ) the total Hamiltonian, using the relative nuclear coordinate  $R$  is effectively three-dimensional and reads:

$$H = \sum_{i=1,2} \left[ -\frac{\nabla_{r_i}^2}{2} + V_{en}(r_i, R) \right] - \frac{\nabla_R^2}{2\mu} + W_{ee}(r_1, r_2) + W_{nn}(R) \quad (1)$$

with

$$V_{en}(r_i, R) = \frac{-2}{\sqrt{(r_i - (1 - \alpha)R)^2 + 1}} - \frac{e^{-\frac{\sqrt{(r_i + \alpha R)^2 + a_{en}}}{\lambda_{en}}}}{\sqrt{(r_i + \alpha R)^2 + a_{en}}} \quad (2)$$

$$W_{ee}(r_1, r_2) = \frac{1}{\sqrt{(r_1 - r_2)^2 + 1}} \quad (3)$$

$$W_{nn}(R) = \frac{e^{-\frac{\sqrt{R^2 + a_{nn}}}{\lambda_{nn}}}}{\sqrt{R^2 + a_{nn}}} \quad (3)$$

and the parameters  $a_{en} = a_{nn} = 0.4$  a.u.,  $\lambda_{en} = 2$  a.u.,  $\lambda_{nn} = 4$  a.u. The reduced mass  $\mu = m_2 m_1 / (m_1 + m_2) = 2754.2292$  a.u. and the ratio  $\alpha = m_1 / (m_1 + m_2) = 1/4$ .

## II. EXACT CALCULATION

The exact results are obtained by propagating the coefficients  $C_j(R; t)$  from the Born-Huang expansion of the full wavefunction:

$$\Psi(r, R; t) = \sum_j C_j(R; t) \Phi_{R,j}^{\text{BO}}(r) \quad (4)$$

using

$$i\partial_t C_i(R; t) = \varepsilon_i^{\text{BO}}(R) C_i(R; t) - \frac{1}{2\mu} \Delta_R C_i(R; t) - \frac{1}{\mu} \sum_j C_j(R; t) d_{i,j}^1 \nabla_R C_j(R; t) - \frac{1}{2\mu} d_i^2 C_i(R; t) \quad (5)$$

where  $d^1$  and  $d^2$  are first and second order non-adiabatic couplings, respectively. We used an  $R$  grid from 0 to 12a.u. with 1000 points and the propagation is done using a time-dependent Lanczos with a Krylov space of size 5 and  $dt = 0.1$ . Spatial differential operators are computed using finite-difference methods of order 8. The BO PES  $\varepsilon_i^{\text{BO}}(R)$  is computed by diagonalizing the matrix of the exact electronic Hamiltonian for 2 electrons on a  $r$  grid from  $-8$  to  $13$  and using 80 points. Convergence with respect to the numerical parameters has been tested.

## III. EHRENFEST CALCULATIONS

See main text for the set of equations. The classical part of the calculation uses 100 Ehrenfest trajectories propagated using a velocity Verlet algorithm and the same time-step  $dt$  as the electronic part (see below).

### A. Electronic part: linear response

The linear-response BO PESs are computed with 600 points from  $-30$  to  $30$  in the  $r$  direction and obtained for each point of an  $R$  grid of 241 points. The electronic propagation uses a direct diagonalization of the Hamiltonian in the subspace of the first three BO states with  $dt = 0.1$ .

### B. Electronic part: real time

The Kohn-Sham equations are propagated using the split operator method on a  $r$  grid with reflecting boundary conditions, a number of points ranging from 200 to 800, and a  $dt$  from 0.1 to 0.01. The parameters have been chosen depending on the convergence of the propagation using a given approximation.

#### IV. MOVIES

As part of supplementary material, we provide the following two movies:

1. **movie\_exact\_exeher\_tdaexx\_tdlraexx\_ne\_nn.mp4** Upper panel: evolution of the nuclear trajectories for the LR and and RT AEXX Ehrenfest calculations as well as the exact nuclear wave packet (see legend). Lower panel are the corresponding electronic densities.
2. **movie\_exact\_exeher\_tdalda\_tdlralda\_ne\_nn.mp4** Upper panel: evolution of the nuclear trajectories for the LR ALDA, RT ALDA and RT ALSD Ehrenfest calculations as well as the exact nuclear wave packet (see legend). Lower panel are the corresponding electronic densities.
3. **movie\_exact\_tdalda\_tdaexx\_ne\_vs\_vext.mp4** Time evolution of the electronic densities and corresponding  $v_s$  and  $v_{\text{ext}}$  potential as well as their spin decomposition when relevant for: RT ALDA, LR ALDA, RT LSD (upper panel); RT AEXX, LR AEXX (lower panel). As a reference, the exact electronic density is show in both panels.
